# Supplementary material for: Electron-electrolyte coupling in AC transport through nanofluidic channels
Source: arXiv:2505.02478 ancillary file (2026-02-24)
Supplement: Supplementary file 1 [file SM.pdf]

Supplementary Material for:

# Electrons as intermediate charge carriers in ion transport through nanoscale channels

Baptiste Coquinot[1,2], Mathieu Lizée[1,3], Lydéric Bocquet[1], and Nikita Kavokine*[4]

[1]Laboratoire de Physique de l'École Normale Supérieure, ENS, Université PSL, CNRS, Sorbonne Université, Université Paris Cité, 24 rue Lhomond, 75005 Paris, France
[2]Institute of Science and Technology Austria (ISTA), Am Campus 1, 3400 Klosterneuburg, Austria
[3]Present address: Fritz Haber Institute of the Max Planck Society, Faradayweg 4-6, 14195 Berlin, Germany
[4]The Quantum Plumbing Lab (LNQ), École Polytechnique Fédérale de Lausanne (EPFL), Station 6, CH-1015 Lausanne, Switzerland

May 5, 2025

## 1 Modified Telegrapher's equation and solutions

Along the propagation lines, the electric potential varies due to the resistivity:

$$L\partial_x U_i(x) = R_i I_i(x) \tag{1}$$

and

$$L\partial_x U_e(x) = R_e I_e(x) = R_e(I - I_i(x)) \tag{2}$$

In the meantime, the difference of potential between the two propagation lines is controlled by the interfacial capacity:

$$U_i(x) - U_e(x) = Z_{\text{EDL}} L\partial_x I_i(x) \tag{3}$$

Thus, we obtain a equation for the ionic current:

$$Z_{\text{EDL}} L^2 \partial_x^2 I_i(x) = (R_i + R_e) I_i(x) - R_e I \tag{4}$$

We denote $I_i^0 = \frac{R_e}{R_i + R_e} I$ the uniform solution corresponding to a system of parallel impedances, and $J = I_i - I_i^0$ the discrepancy from the uniform solution. Therefore, we obtain the modified Telegrapher's equation (Eq. (1) of the main text):

$$\ell(\omega)^2 \partial_x^2 J(x,\omega) = 2iJ(x,\omega) \tag{5}$$

where $\ell$ is the exchange length defined in Eq. (2) of the main text.

In general, we consider symmetric entrance impedances $Z_i^{\text{in}}$ (resp. $Z_e^{\text{in}}$) at the edges of the transmission line $x = \pm L/2$. This sets the boundary conditions:

$$U_i - U_e = \mp Z_i^{\text{in}} I_i \pm Z_e^{\text{in}}(I - I_i) = Z_{\text{EDL}} L\partial_x I_i \tag{6}$$

*i.e.*

$$\mp Z_{\text{EDL}} L\partial_x J - (Z_i^{\text{in}} + Z_e^{\text{in}})J = \frac{R_e Z_i^{\text{in}} - R_i Z_e^{\text{in}}}{R_i + R_e} I \tag{7}$$

*nikita.kavokine@epfl.ch

Thus,

$$J(x) = \frac{(\zeta_e - \zeta_i)R_iR_e}{(R_i+R_e)^2} \frac{\cosh((1+i)x/\ell)}{(1-i)\frac{\ell}{2L}\sinh((1+i)L/2\ell) + \zeta_{\rm tot}\cosh((1+i)L/2\ell)} I \tag{8}$$

where

$$\zeta_{\rm tot} = \frac{Z_i^{\rm in} + Z_e^{\rm in}}{R_i + R_e}, \qquad \zeta_i = \frac{Z_i^{\rm in}}{R_i}, \qquad \zeta_e = \frac{Z_e^{\rm in}}{R_e} \tag{9}$$

compare the entrance impedances with the bulk resistance. The total difference of potential throughout the system can be computing following the ionic path:

$$\Delta U = 2Z_i^{\rm in} I_i(\pm L/2) + \frac{\rho_i}{W}\int {\rm d}x\, I_i(x) \tag{10}$$

Recalling that $I_i(x) = I_i^0 + J(x)$, we obtain:

$$Z = \frac{\Delta U}{I} = \frac{R_iR_e}{R_i+R_e}(1+2\zeta_i) + \frac{(\zeta_e - \zeta_i)R_iR_e}{(R_i+R_e)^2}\frac{2Z_i^{\rm in} + (1-i)\frac{\ell}{L}R_i\tanh\left((1+i)\frac{L}{2\ell}\right)}{\zeta_{\rm tot} + (1-i)\frac{\ell}{2L}\tanh\left((1+i)\frac{L}{2\ell}\right)} \tag{11}$$

Introducing the complex step function

$$F(x) = \frac{\tanh[(1+i)x]}{(1+i)x} \tag{12}$$

such that $F(x) \longrightarrow_{x\to 0} 1$ and $F(x) \sim_{x\to\infty} \frac{1}{(1+i)x} \longrightarrow 0$, and simplifying Eq. (11), we obtain:

$$Z = \frac{R_iR_e}{R_i+R_e}\frac{2\zeta_{\rm tot} + 4\zeta_i\zeta_e + \left(1 + 2\frac{\zeta_iR_e + \zeta_eR_i}{R_i+R_e}\right)F\left(\frac{L}{2\ell}\right)}{2\zeta_{\rm tot} + F\left(\frac{L}{2\ell}\right)} \tag{13}$$

Measuring the ionic current through a metallic channel then corresponds to the limit $Z_e^{\rm in} = \infty$. If we do not focus on the effect of the ionic electrode, then we can also take $Z_i^{\rm in} = 0$.

For asymmetric boundary conditions, Eq. (6) remains valid with asymmetric entrance impedances. For instance, if we use on one side an electronic electrode and on the side side an ionic electrode, it corresponds to $Z_i^{\rm in} = 0$ and $Z_e^{\rm in} = \infty$ at $x = -L/2$, and $Z_e^{\rm in} = 0$ and $Z_i^{\rm in} = \infty$ at $x = +L/2$. In practice for the ionic current, these boundary conditions become $J(-L/2) = r_iI$ and $J(L/2) = -r_eI$. Following the same steps, we then obtain:

$$Z = \frac{R_iR_e}{R_i+R_e} + (R_i+R_e)\left[\frac{1}{4}\frac{(R_i-R_e)^2}{(R_i+R_e)^2}F(L/2\ell) + \frac{1}{2i}\left(\frac{\ell}{L}\right)^2 F(L/2\ell)^{-1}\right] \tag{14}$$

Let us now consider the case of two ionic electrodes measuring the ionic current through a closed channel. This corresponds to twice the previous circuit, of length $L/2$, in series. Thus, we directly obtain Eq. (6) of the main text.
